# Supplementary material for: Comparative validation of surgical phase recognition, instrument keypoint estimation, and instrument instance segmentation in endoscopy: Results of the PhaKIR 2024 challenge
Source: arXiv:2507.16559 ancillary file (2026-01-19)
Supplement: Supplementary file 1 [file Supplement_S1.pdf]

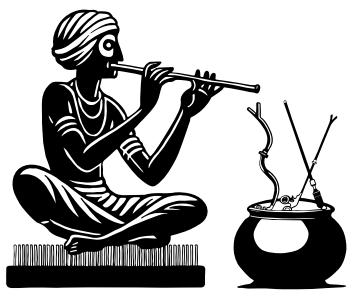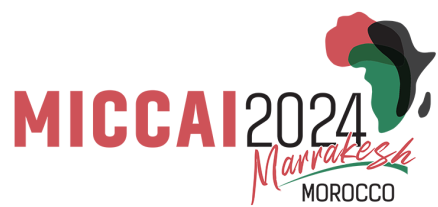

# **PhaKIR Challenge - Phase, Keypoint and Instrument Recognition *Data Description and Labeling Instructions***

**Part of the Endoscopic Vision (EndoVis) Challenge at MICCAI 2024**

Website: <https://phakir.re-mic.de/>

E-Mail: [phakir2024@re-mic.de](mailto:phakir2024@re-mic.de)

Organization:

Regensburg Medical Image Computing (ReMIC) Lab

Website: <https://re-mic.de/>

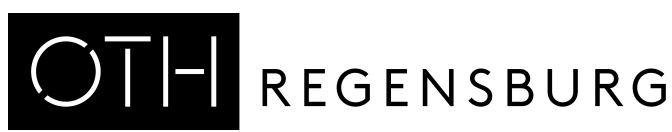

# Contents

- 1 General 2**
  - 1.1 Introduction . . . . . 2
  - 1.2 Structure of this Document . . . . . 2
  - 1.3 Structure of the Dataset . . . . . 2
  - 1.4 Video Distribution . . . . . 3
- 2 Procedure Phase Recognition 4**
  - 2.1 Data Description . . . . . 4
  - 2.2 Labeling Instructions . . . . . 4
- 3 Keypoint Estimation 5**
  - 3.1 Data Description . . . . . 5
  - 3.2 Labeling Instructions . . . . . 8
- 4 Instrument Instance Segmentation 9**
  - 4.1 Data Description . . . . . 9
  - 4.2 Labeling Instructions . . . . . 11

# 1 General

## 1.1 Introduction

Accurate and reliable recognition and localization of surgical instruments in endoscopic video recordings is the basis for a variety of applications in computer- and robot-assisted minimally invasive surgery (RAMIS) [1]. To process the information extracted from the endoscopic images in the best possible way, the inclusion of the context of the operation can be used as a promising possibility, which can be realized, for example, by knowing the current phase of an intervention.

In our EndoVis2024 (<https://opencas.dkfz.de/endovis/challenges/2024/>) sub-challenge, we present a dataset for which three tasks are to be performed: Instance segmentation of the surgical instruments, keypoint estimation, and procedure phase recognition. The following annotations are available for this: pixel-accurate instance segmentations of surgical instruments together with their instrument types for a total of 19 categories, coordinates of relevant instrument keypoints (instrument tip(s), shaft-tip transition, shaft), and a classification of the phases of an intervention into eight different phase categories.

In addition to existing datasets, our annotations provide instance segmentations of surgical instruments, relevant keypoints, and intervention phases in one dataset and thus comprehensively cover instrument localization and the context of the operation. Furthermore, the provision of the complete video sequences offers the opportunity to include the temporal information regarding the respective tasks and thus further optimize the resulting methods and outcomes.

## 1.2 Structure of this Document

This document is structured as follows. Chapter 1 provides an overview of the overall task and describes the structure of the provided dataset. The Chapters 2, 3, and 4 describe the three tasks of the challenge in more detail, namely procedure phase recognition, keypoint estimation, and instrument instance segmentation. For each of the three tasks, the structure of the provided data is presented and information on how this data is annotated is described, together with examples.

## 1.3 Structure of the Dataset

For each training video provided, there exists a zip archive that can be downloaded from the data page (<https://phakir.re-mic.de/data/>) after successful registration and login to the challenge website. This zip-archive provides the following data, with the number of an arbitrary video being designated as XX:

- `Video_XX.mp4`: Video file of the operation, which can be split into the individual frames using the script `split_video_in_frames.py`.
- `Video_XX_Phases.csv`: Indication of the current phase of the procedure for each individual frame.
- `Video_XX_Keypoints.json`: Specification of the number, types, and locations of the keypoints for the interval of one frame per second.
- `Video_XX_Masks.zip`: Color-coded segmentation masks for the interval of one frame per second.
- `Video_XX_Cuts.csv`: Indication of the frame numbers where sequences are cut out due to the anonymization of the recordings. This information is particularly interesting when using the temporal information, for example, to reset modules at this point that take the temporal component into account.

In addition, a script (`split_video_in_frames.py`) is provided with which the video sequences can be separated into individual frames and stored on the hard disk. This script can be executed with the command: `python split_video_in_frames.py XX`. It creates a PNG file for each frame using the OpenCV library [2], whereby the value six is used as the compression level. Valid values for the compression level are integer values in the interval  $[0,9]$ . A higher value results in a smaller file size and a longer saving time, a lower value speeds up saving but requires more storage space.<sup>1</sup> The script can be modified at any time and adapted to personal preferences, for example with regard to the compression level or other components.

### 1.4 Video Distribution

We provide an overall of 13 videos originating from three hospitals, with the following distribution of training and test videos:

- Training:
  - Hospital 1: 6 Videos
  - Hospital 2: 1 Video
  - Hospital 3: 1 Video
- Test:
  - Hospital 1: 3 Videos
  - Hospital 2: 1 Video
  - Hospital 3: 1 Video

---

<sup>1</sup>[https://docs.opencv.org/3.4/d8/d6a/group\\_\\_imgcodecs\\_\\_flags.html](https://docs.opencv.org/3.4/d8/d6a/group__imgcodecs__flags.html)

## 2 Procedure Phase Recognition

In the following, the annotations for the phases of a surgical procedure are described, as well as the instructions for the creation of these annotations.

### 2.1 Data Description

For the annotation of the surgical phases, we follow the phase designations of the famous Cholec80 dataset [3]. In addition, we introduce a category “undefined”, which describes the frames that are localized between two phases and in which no actions are performed that can be assigned to one of the other phases. This leads to the following phase definitions:

- P0: Undefined
- P1: Preparation
- P2: Calot triangle dissection
- P3: Clipping and cutting
- P4: Gallbladder dissection
- P5: Gallbladder packaging
- P6: Cleaning and coagulation
- P7: Gallbladder retraction

### 2.2 Labeling Instructions

To create the procedure phase annotations, the video sequences of the operations are analyzed, and all individual frames are divided into one of the seven categories P1 - P7 described above based on the actions performed. Phases in which none of these actions are performed, such as the transition from one phase to the next, are designated as phase: “P0: Undefined”. The result is a file in which the corresponding phase is specified for each individual frame.

## 3 Keypoint Estimation

In the following, the annotations for the number, types, and locations of the instrument keypoints are described, as well as the instructions for the creation of these annotations.

### 3.1 Data Description

Annotations for instrument keypoints are available for one frame per second, with the intermediate frames being made available without annotations. The number of keypoints depends on the instrument class. Instruments whose tip can be opened, for example, to grasp or cut something, and which are made up of two parts (shaft and tip) have four keypoints annotated, namely one keypoint for each part of the tip (Tip, Tip), one keypoint for the transition between tip and shaft (ShaftPoint), and one keypoint that describes the end of the instrument at the edge of the image (EndPoint). Tools that also consist of the two parts shaft and tip and whose tip cannot be opened have three keypoints, whereby the tip of the instrument is described by only one keypoint instead of two. Instruments where it is not possible to distinguish between the tip and shaft or where there is no delimitation between both parts have two keypoints, one for the tip and one EndPoint. An assignment of instrument categories to keypoint classes can be found in the following list:

- 4 Keypoints (Tip, Tip, ShaftPoint, EndPoint):
  - Bipolar-Clamp
  - Blunt-Grasper
  - Blunt-Grasper-Curved
  - Blunt-Grasper-Spec.
  - Clip-Applicator
  - Grasper
  - Hook-Clamp
  - Overholt
  - PE-Forceps
  - Scissor
  - Sponge-Clamp
- 3 Keypoints (Tip, ShaftPoint, EndPoint):
  - Argonbeamer
  - Dissection-Hook

### 3 Keypoint Estimation

- HFcoag-Probe
- Suction-Rod
- 2 Keypoints (Tip, EndPoint):
  - Drainage
  - Needle-Probe
  - Palpation-Probe
  - Trocar-Tip

The structure of the JSON document containing the annotated keypoints is shown in Listing 1. All available instrument labels are listed under the `categories` object. The `items` object describes a list where each entry corresponds to the annotations of the keypoints in exactly one corresponding frame, which is indicated by the `id` attribute.

**Listing 1:** Structure of the JSON document that contains the annotated keypoints.

```

1 {
2   "categories": {
3     "label": {
4       "labels": [
5         {
6           "name": "KP-Clip-Applicator"
7         },
8         ...,
9         {
10          "name": "KP-Bipolar-Clamp"
11        }
12      ],
13      "attributes": [
14        "Point_Class"
15      ]
16    },
17  },
18  "items": [
19    {
20      "id": "frame_000125",
21      "annotations": [
22        {
23          "label_id": 1,
24          "keypoints": [
25            {
26              "point_class": "Tip",
27              "visibility": 2,
28              "coordinates": [
29                540,
30                774
31              ]
32            }
33          ]
34        },
35        ...
36      ]
37    }
38  ]

```

For each existing instrument in a frame, the `label_id` indicates the tool category, which corresponds to the index of the instrument in the `labels` list located in the `categories` object. All keypoints of the instrument are listed under the `keypoints` list. For each annotated keypoint, the value of the `visibility` property indicates if a keypoint is annotated and visible (`visibility = 2`), annotated and occluded or hidden (`visibility = 1`), or not annotated because it is not located inside the frame or in case

it is not possible to estimate its position accurately (`visibility = 0`). This procedure is based on the one described in the Common Objects in Context (COCO) dataset (<https://cocodataset.org/#keypoints-eval>). The values in the coordinates list specify the x- and y-coordinate of each keypoint, with the origin of the coordinate system at the top left of the image.

## 3.2 Labeling Instructions

The annotations for the keypoints are created in a semi-automated process based on the segmentation masks by using an algorithm to generate the best possible labels for the position of the keypoints and then adjusting them manually, as well as manually defining the visibility of the keypoints.

The categories of the keypoints result from the defined classes within the segmentation masks. For the `EndPoint` of an instrument there is always an annotation, i.e., the `visibility` attribute for this point can only take the values `visibility = 1` or `visibility = 2`. The `EndPoint` and `ShaftPoint` of a surgical tool are placed so that they describe the actual center of the physical instrument, not just the center of the visible area. The keypoints for the tips of an instrument are positioned in such a way so that they best describe the center of the relevant tip structure.

The entire video sequences are available to the annotators for both the training and the test data, i.e., frames from the past and the future can also be included for the precise localization of the keypoints. The presumed and estimated movements of the instruments over time can thus be used to determine the keypoints as accurately as possible.

# 4 Instrument Instance Segmentation

In the following, the annotations for the instance segmentation of the surgical instruments are described, as well as the instructions for the creation of these annotations.

## 4.1 Data Description

One pixel in a frame always corresponds to exactly one instrument or to the background, and the individual instruments within a frame are separated by different colors. The red (R) and green (G) channels define the class of the instrument, and the blue (B) channel describes the instance of an object within an instrument class. For example, if there are two objects in a frame corresponding to one instrument class, the values of the R and G channels of both objects are identical, and the value of the B channel is different. An overview of the various instrument classes and the associated color codes in RGB format is provided in Table 1, where the B value for an arbitrary instance is specified for each class.

**Table 1:** Overview of the various instrument classes and the associated color codes in RGB format, where the value of the B channel for an arbitrary instance is specified for each class. If several instances of an instrument occur in a frame, there are several segmentations with identical R and G values, but different B values.

| Nr. | Label                | RGB-Encoding    | Visualization                                                                         |
|-----|----------------------|-----------------|---------------------------------------------------------------------------------------|
| 1   | Argonbeamer          | [60, 50, 50]    | 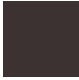 |
| 2   | Bipolar-Clamp        | [89, 134, 179]  | 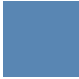 |
| 3   | Blunt-Grasper        | [128, 128, 128] | 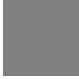 |
| 4   | Blunt-Grasper-Curved | [200, 102, 235] | 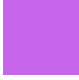 |
| 5   | Blunt-Grasper-Spec.  | [179, 102, 235] | 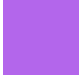 |
| 6   | Clip-Applicator      | [0, 0, 255]     | 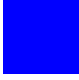 |

Table 1: continued.

| Nr. | Label                | RGB-Encoding    | Visualization                                                                         |
|-----|----------------------|-----------------|---------------------------------------------------------------------------------------|
| 7   | Dissection-Hook      | [80, 140, 0]    | 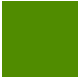   |
| 8   | Drainage             | [255, 100, 0]   | 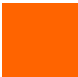   |
| 9   | Grasper              | [255, 130, 0]   | 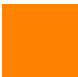   |
| 10  | HF-Coagulation-Probe | [255, 0, 153]   | 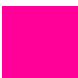   |
| 11  | Hook-Clamp           | [0, 80, 80]     | 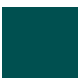   |
| 12  | Needle-Probe         | [204, 153, 153] | 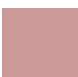   |
| 13  | Overholt             | [255, 200, 170] | 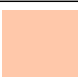  |
| 14  | Palpation-Probe      | [255, 102, 255] | 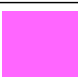 |
| 15  | PE-Forceps           | [30, 144, 1]    | 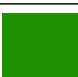 |
| 16  | Scissor              | [255, 255, 0]   | 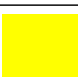 |
| 17  | Sponge-Clamp         | [40, 120, 80]   | 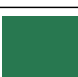 |
| 18  | Suction-Rod          | [153, 0, 204]   | 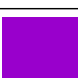 |
| 19  | Trocar-Tip           | [153, 102, 0]   | 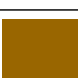 |

## 4.2 Labeling Instructions

The visible instruments within a frame are defined by manually created contours, whereby the area within a contour describes the area of an instrument.

Analogous to the annotation of the keypoints, the entire video sequences are available to the annotators for both the training and the test data, i.e., frames from the past and the future can also be included for the segmentation of the surgical instruments. In contrast to the keypoint annotations, however, only pixels of actually visible instruments are annotated, i.e., no assumptions or estimates are made as to how objects might move. To ensure consistency regarding the manual segmentation of the surgical tools, a number of rules is defined, which are applied by the annotators:

1. *Unique segmentations*: Each pixel of a frame corresponds to exactly one class, either to one of the instrument classes listed in Table 1, or to the background. Only the visually visible parts of the instruments are segmented, i.e., no estimation or assumption is made regarding the probable movement of an instrument or its presumed position if it is obscured by other objects.
2. *Relevant objects*: Only the surgical instruments listed in Table 1 are segmented and no distinction is made between shaft and tip, instead the instruments are segmented as a whole. Other structures such as tissue, clips, organs, etc. are not taken into account and are considered as background.
3. *Occlusions*: If there are several instruments on top of each other or if instruments are covered by organs, tissue, blood, clips, etc., the area that is closest to the endoscope determines the category, and areas that are further away from the camera are accordingly regarded as background. If an instrument is partially obscured, its segmentation mask can consist of several parts that have the same color encoding. In the case of extreme smoke development, which impairs the view to such an extent that a certain instrument can no longer be recognized, the smoke is also regarded as an overlay and the area is annotated as background.
4. *Holes in instruments*: If there are holes within an instrument, i.e., areas within the instrument that are completely surrounded by the surface of the instrument based on the actual instrument structure, the area of these holes is considered to be part of the instrument. The only exception is the trocar, through which the endoscope is introduced into the abdominal cavity when it is only partially visible. In this case, the area inside the trocar is not regarded as an instrument hole, but as the camera's field of view.
5. *(Motion) blur*: In the case of blurred areas, for example, due to the very fast movement of an instrument or a smeared endoscope view, the actually visible area of an instrument is segmented as accurately as possible.
6. *Instrument instance categorization*: As shown in Table 1, the R and G channels of a segmented area describe the class of the instrument, and the B channel indicates the instance within this class. If an instrument class occurs twice in a frame, the corresponding segmentations have identical R and G channel values, but a different B value in order to distinguish the object instances.

In the following Table 2, these rules are visualized using various examples, with the original frame on the left and the corresponding color-coded segmentation mask on the

right. In addition, a brief explanation is given for each example to explain which rules are applied and should be illustrated in the specific case.

**Table 2:** Visualization of exemplary frames together with the corresponding color-coded segmentation masks resulting from the application of the abovementioned rules.

| Frame                                                                                                                                                                                                                                                                                                                                                                                                                                                   | Segmentation Mask                                                                    |
|---------------------------------------------------------------------------------------------------------------------------------------------------------------------------------------------------------------------------------------------------------------------------------------------------------------------------------------------------------------------------------------------------------------------------------------------------------|--------------------------------------------------------------------------------------|
| 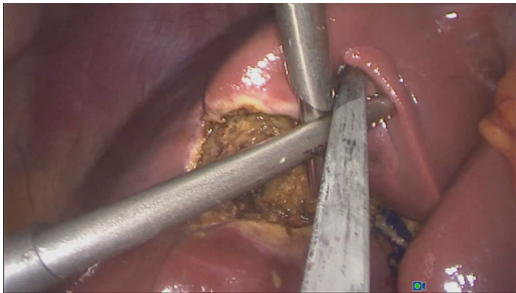                                                                                                                                                                                                                                                                                                                                                                       | 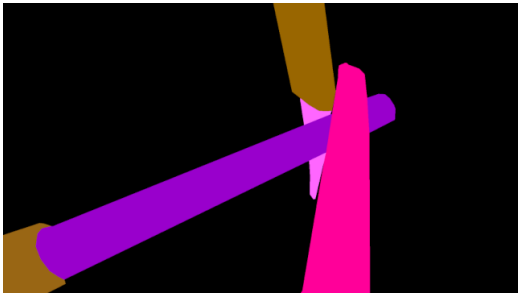   |
| <p><i>Example 1:</i> Each pixel corresponds to exactly one instrument or to the background (rule 1). The order of the superimposed instruments is determined by their distance from the endoscope, and the class closest to the camera is selected for each pixel (rule 3). The frame shows two trocars whose pixels have identical R and G channels, while the B channel differs by 20 units in order to distinguish different instances (rule 6).</p> |                                                                                      |
| 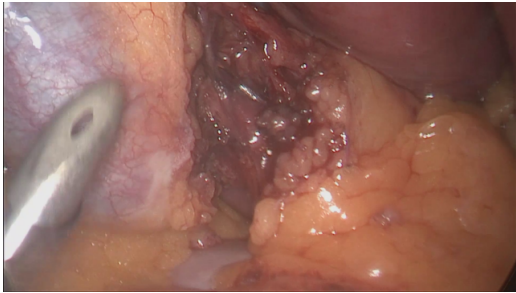                                                                                                                                                                                                                                                                                                                                                                      | 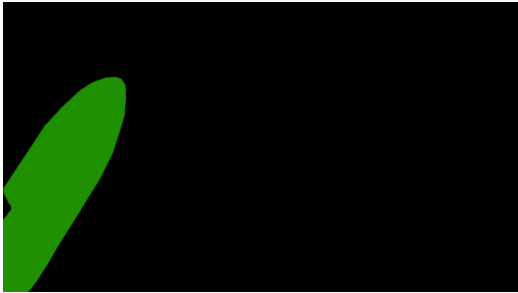  |
| <p><i>Example 2:</i> The hole in the PE-Forceps is not excluded, but is considered part of the instrument (rule 4). The part of the instrument that is clearly visible despite the motion blur is annotated (rule 5).</p>                                                                                                                                                                                                                               |                                                                                      |
| 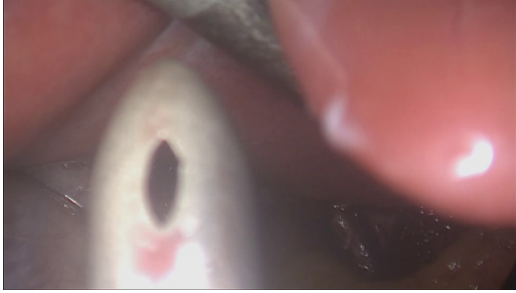                                                                                                                                                                                                                                                                                                                                                                     | 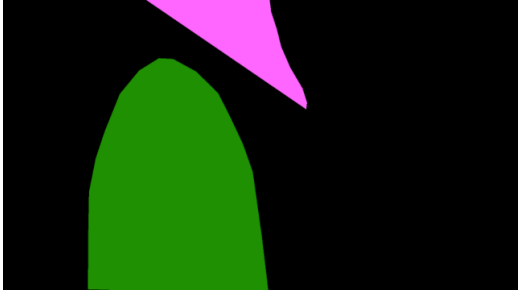 |
| <p><i>Example 3:</i> The hole in the PE-Forceps is not excluded, but is considered part of the instrument (rule 4). Only the visible part of the occluded Palpation-Probe is annotated (rule 3).</p>                                                                                                                                                                                                                                                    |                                                                                      |

Table 2: continued.

| Frame                                                                                                                                                                                                                                                                                                                                                                                                                   | Segmentation Mask                                                                    |
|-------------------------------------------------------------------------------------------------------------------------------------------------------------------------------------------------------------------------------------------------------------------------------------------------------------------------------------------------------------------------------------------------------------------------|--------------------------------------------------------------------------------------|
| 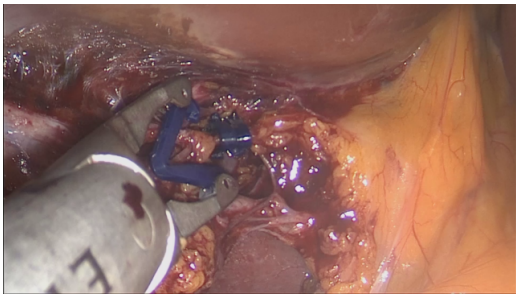                                                                                                                                                                                                                                                                                                                                       | 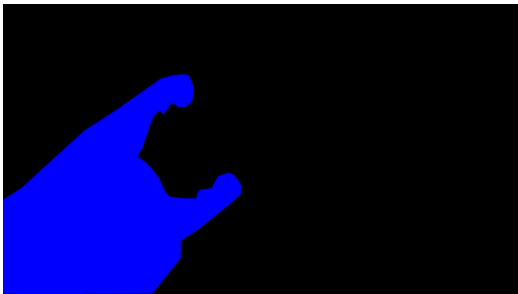   |
| <p>Example 4: Only the relevant area covered by the Clip-Applicator is annotated, the clips are not considered as part of the instrument (rule 2).</p>                                                                                                                                                                                                                                                                  |                                                                                      |
| 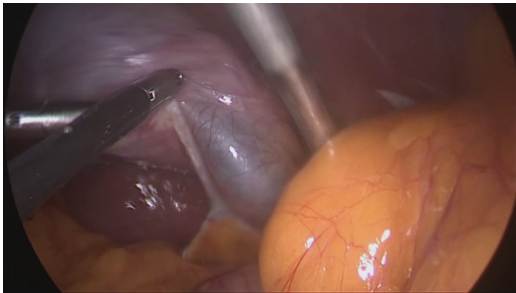                                                                                                                                                                                                                                                                                                                                      | 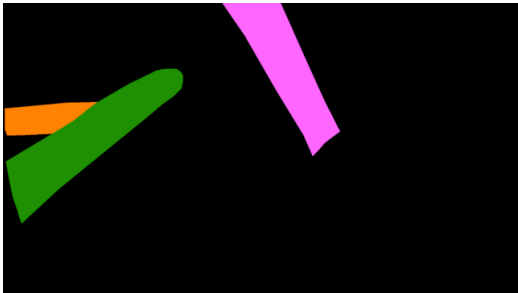  |
| <p>Example 5: At the left edge of the image, only the visible part of the PE-Forceps is annotated, and no assumptions are made about the structure outside the visible area (rule 1). Only the visible part of the occluded Palpation-Probe is annotated, and since the PE-Forceps is located closer to the endoscope, the pixels overlapping with the Grasper are considered to belong to the PE-Forceps (rule 3).</p> |                                                                                      |
| 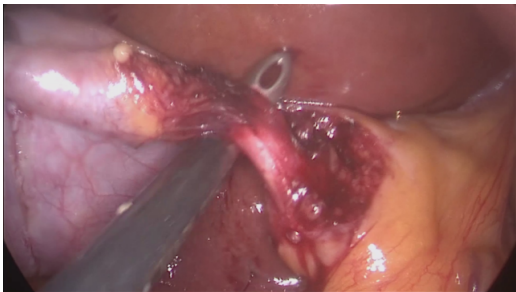                                                                                                                                                                                                                                                                                                                                     | 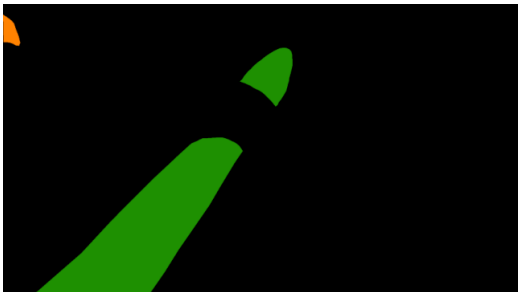 |
| <p>Example 6: Due to partial occlusion of the PE-Forceps by tissue, the segmentation consists of two parts with identical color encoding (rule 3).</p>                                                                                                                                                                                                                                                                  |                                                                                      |

Table 2: continued.

| Frame                                                                                                                                                                                                                                                                                                                                                                                                                                           | Segmentation Mask                                                                    |
|-------------------------------------------------------------------------------------------------------------------------------------------------------------------------------------------------------------------------------------------------------------------------------------------------------------------------------------------------------------------------------------------------------------------------------------------------|--------------------------------------------------------------------------------------|
| 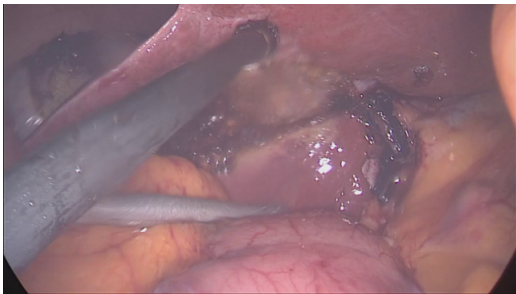                                                                                                                                                                                                                                                                                                                                                               | 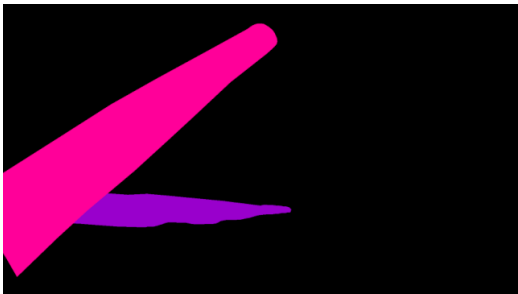   |
| <p><i>Example 7:</i> At the lower left corner of the image, only the visible part of the HFcoag-Probe is annotated, and no assumptions are made about the structure outside the visible area (rule 1). Only the visible part of the occluded Suction-Rod is annotated (rule 3). Because the HFcoag-Probe is located closer to the endoscope than Suction-Rod, the associated pixels are assigned to the class of the HFcoag-Probe (rule 3).</p> |                                                                                      |
| 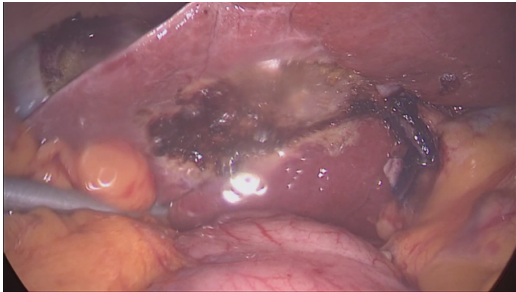                                                                                                                                                                                                                                                                                                                                                              | 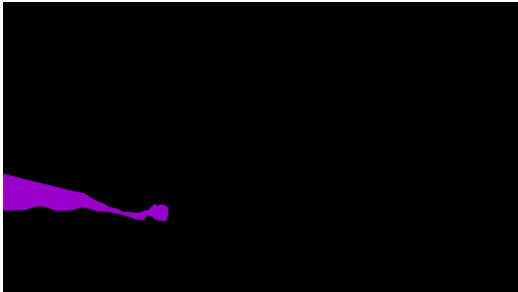  |
| <p><i>Example 8:</i> Only the visible part of the occluded Suction-Rod is annotated, and the partial occlusion caused by tissue is not considered (rule 3).</p>                                                                                                                                                                                                                                                                                 |                                                                                      |
| 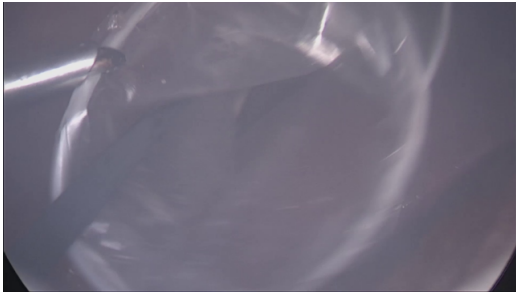                                                                                                                                                                                                                                                                                                                                                             | 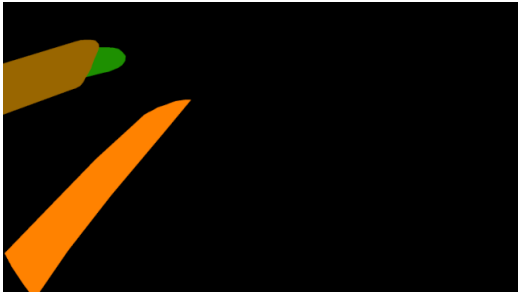 |
| <p><i>Example 9:</i> At the lower left corner of the image, only the visible part of the Grasper is annotated, and no assumptions are made about the structure outside the visible area (rule 1). Only the visible part of the occluded PE-Forceps is annotated, and the partial occlusion caused by the plastic bag is not considered (rule 3).</p>                                                                                            |                                                                                      |

Table 2: continued.

| Frame                                                                                                                                                                                                                                                                                                                                                         | Segmentation Mask                                                                  |
|---------------------------------------------------------------------------------------------------------------------------------------------------------------------------------------------------------------------------------------------------------------------------------------------------------------------------------------------------------------|------------------------------------------------------------------------------------|
| 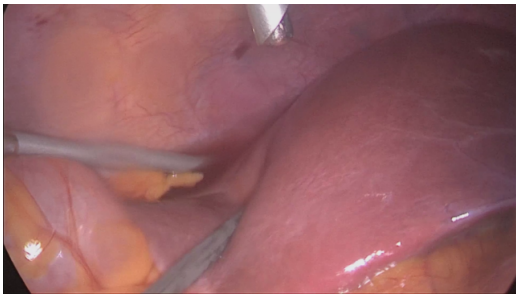                                                                                                                                                                                                                                                                             | 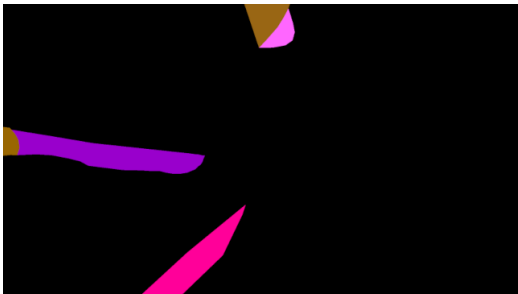 |
| <p>Example 10: Only the visible part of the occluded Suction-Rod and HFcoag-Probe is annotated, and the partial occlusion caused by tissue and organs is not considered (rule 3). The frame shows two trocars whose pixels have identical R and G channels, while the B channel differs by 20 units in order to distinguish different instances (rule 6).</p> |                                                                                    |

## References

- [1] Tobias Rueckert, Daniel Rueckert, and Christoph Palm. “Methods and datasets for segmentation of minimally invasive surgical instruments in endoscopic images and videos: A review of the state of the art”. In: *Computers in Biology and Medicine* 169 (2024), pages 107929–107929. DOI: <https://doi.org/10.1016/j.combiomed.2024.107929> (cited on page 2).
- [2] Gary Bradski. “The OpenCV Library.” In: *Dr. Dobb’s Journal: Software Tools for the Professional Programmer* 25.11 (2000), pages 120–123 (cited on page 3).
- [3] Andru P Twinanda, Sherif Shehata, Didier Mutter, Jacques Marescaux, Michel De Mathelin, and Nicolas Padoy. “EndoNet: A Deep Architecture for Recognition Tasks on Laparoscopic Videos”. In: *IEEE Transactions on Medical Imaging* 36.1 (2016), pages 86–97. DOI: <https://doi.org/10.1109/TMI.2016.2593957> (cited on page 4).
