# Supplementary material for: Comparative validation of surgical phase recognition, instrument keypoint estimation, and instrument instance segmentation in endoscopy: Results of the PhaKIR 2024 challenge
Source: arXiv:2507.16559 ancillary file (2026-01-19)
Supplement: Supplementary file 2 [file Supplement_S2.pdf]

# PhaKIR: Surgical Procedure Phase Recognition, Keypoint Estimation, and Instrument Instance Segmentation

## SUMMARY

### Abstract

Provide a summary of the challenge purpose. This should include a general introduction in the topic from both a biomedical as well as from a technical point of view and clearly state the envisioned technical and/or biomedical impact of the challenge.

Accurate and reliable recognition and localization of surgical instruments in endoscopic video recordings is the basis for a variety of applications in computer- and robot-assisted minimally invasive surgery (RAMIS), such as surgical training systems, surgical skill assessment, or autonomous endoscope guidance. The robust handling of real-world conditions such as varying illumination levels, blurred movement of the instruments and the camera, severe sudden bleeding that impairs the field of view, or even unexpected smoke development is an important prerequisite for such procedures. To process the information extracted from the endoscopic images in the best possible way, the inclusion of the context of the operation can be used as a promising possibility, which can be realized, for example, by knowing the current phase of an intervention.

In our subchallenge, we present a dataset for which three tasks are to be performed: Instance segmentation of the surgical instruments, keypoint estimation, and procedure phase recognition. The following annotations are available for this: pixel-accurate instance segmentations of surgical instruments together with their instrument types, of which a total of 20 categories are distinguished, coordinates of relevant instrument keypoints (instrument tip(s), shaft-tip transition, shaft), and a classification of the phases of an intervention into seven different phase categories. Our dataset consists of 13 individual real-world videos of human cholecystectomies ranging from 23 to 60 minutes in duration. The procedures were performed by experienced physicians, and the videos were recorded in three hospitals. In addition to the complete video sequences, we provide annotations in a one-frame-per-second time interval, resulting in approximately 30,000 annotated and 838,000 not annotated frames. In addition to existing datasets, our annotations provide instance segmentations of surgical instruments, relevant keypoints, and intervention phases in one dataset and thus comprehensively cover instrument localization and the context of the operation. We believe that providing our dataset and conducting our subchallenge will contribute to the exploration of new approaches in RAMIS, especially taking temporal information into account, and enrich the community in the field of instrument recognition and phase classification.

### Keywords

List the primary keywords that characterize the task.

Endoscopic Vision, Surgical Instruments, Instance Segmentation, Keypoint Estimation, Phase Recognition

## ORGANIZATION

### Organizers

a) Provide information on the organizing team (names and affiliations).

Tobias Rueckert, Christoph Palm, OTH Regensburg  
 Dirk Wilhelm, Hubertus Feußner, Daniel Rueckert, TU Munich

b) Provide information on the primary contact person.

Tobias Rueckert  
 tobias.rueckert@oth-regensburg.de

### Life cycle type

Define the intended submission cycle of the challenge. Include information on whether/how the challenge will be continued after the challenge has taken place. Not every challenge closes after the submission deadline (one-time event). Sometimes it is possible to submit results after the deadline (open call) or the challenge is repeated with some modifications (repeated event).

Examples:

- One-time event with fixed conference submission deadline
- Open call (challenge opens for new submissions after conference deadline)
- Repeated event with annual fixed conference submission deadline

One-time event with fixed submission deadline.

### Challenge venue and platform

a) Report the event (e.g. conference) that is associated with the challenge (if any).

N/A

b) Report the platform (e.g. grand-challenge.org) used to run the challenge.

Synapse.org and self-hosted individual challenge website

c) Provide the URL for the challenge website (if any).

Synapse.org: In Preparation. Individual challenge website: phakir.re-mic.de

### Participation policies

a) Define the allowed user interaction of the algorithms assessed (e.g. only (semi-) automatic methods allowed).

**Only automatic methods are allowed.**

b) Define the policy on the usage of training data. The data used to train algorithms may, for example, be restricted to the data provided by the challenge or to publicly available data including (open) pre-trained nets.

**Only training data provided by the challenge organizers and publicly available data sets are allowed for training. In addition, networks that have been pre-trained on publicly available datasets may be used.**

c) Define the participation policy for members of the organizers' institutes. For example, members of the organizers' institutes may participate in the challenge but are not eligible for awards.

**Members of the organizing institutes may participate, but are not eligible for awards.**

d) Define the award policy. In particular, provide details with respect to challenge prizes.

There will be three tasks in the challenge (instance segmentation, keypoint estimation and phase recognition). The top three teams per task will be named at the MICCAI 2024 event, and each participating team will receive a certificate confirming their participation and indicating their rank compared to the other methods.

e) Define the policy for result announcement.

Examples:

- Top 3 performing methods will be announced publicly.
- Participating teams can choose whether the performance results will be made public.

The results of all teams will be presented at the MICCAI 2024 EndoVis challenge event. Subsequently, as there is no continuously updated leaderboard, the results of the top three teams for each task will be published on the challenge website and all results of all participants will be included in the joint challenge publication.

f) Define the publication policy. In particular, provide details on ...

- ... who of the participating teams/the participating teams' members qualifies as author
- ... whether the participating teams may publish their own results separately, and (if so)
- ... whether an embargo time is defined (so that challenge organizers can publish a challenge paper first).

All contributing members of each participating team will be listed on the joint challenge publication. The authors of the submitted methods are not allowed to publish any results before the publication of the joint challenge paper. All participating teams will submit a brief methodology report.

### Submission method

a) Describe the method used for result submission. Preferably, provide a link to the submission instructions.

Examples:

- Docker container on the Synapse platform. Link to submission instructions: <URL>
- Algorithm output was sent to organizers via e-mail. Submission instructions were sent by e-mail.

Docker container on the self-hosted challenge website. The Submission instructions are in preparation, a link will be provided. All participating teams have to submit a brief methodology report.

b) Provide information on the possibility for participating teams to evaluate their algorithms before submitting final results. For example, many challenges allow submission of multiple results, and only the last run is officially counted to compute challenge results.

We provide a platform for participants to verify the technical functionality of their submitted Docker containers. For the evaluation of the algorithms, only the last submitted version will be considered. An evaluation on the test data will only be performed once per team to prevent iterative adaptation to the test data.

### Challenge schedule

Provide a timetable for the challenge. Preferably, this should include

- the release date(s) of the training cases (if any)
- the registration date/period

- the release date(s) of the test cases and validation cases (if any)
- the submission date(s)
- associated workshop days (if any)
- the release date(s) of the results

Challenge website and challenge registration opens: April 2024

Release of training data: May 2024

Release of docker submission guide/evaluation instructions: 1st of August 2024

Submission deadline and registration closing: 15th of September 2024 ; Methodology report deadline: 15th of September 2024

Challenge Day: Day of Endovis 2024

### **Ethics approval**

Indicate whether ethics approval is necessary for the data. If yes, provide details on the ethics approval, preferably institutional review board, location, date and number of the ethics approval (if applicable). Add the URL or a reference to the document of the ethics approval (if available).

Only anonymized data collected in an ethically approved research project approved by the local ethics committee of the Technical University of Munich (approval code 337/21 S-EB) is used.

### **Data usage agreement**

Clarify how the data can be used and distributed by the teams that participate in the challenge and by others during and after the challenge. This should include the explicit listing of the license applied.

Examples:

- CC BY (Attribution)
- CC BY-SA (Attribution-ShareAlike)
- CC BY-ND (Attribution-NoDerivs)
- CC BY-NC (Attribution-NonCommercial)
- CC BY-NC-SA (Attribution-NonCommercial-ShareAlike)
- CC BY-NC-ND (Attribution-NonCommercial-NoDerivs)

CC BY-NC-SA

### **Code availability**

a) Provide information on the accessibility of the organizers' evaluation software (e.g. code to produce rankings). Preferably, provide a link to the code and add information on the supported platforms.

The evaluation docker container together with an evaluation script for calculating the metrics will be made available to participants on the challenge website.

b) In an analogous manner, provide information on the accessibility of the participating teams' code.

Participants are encouraged to make the algorithms and their Docker containers publicly available. However, if this is not desired by individual participants or groups, private submissions will also be accepted.

### Conflicts of interest

Provide information related to conflicts of interest. In particular provide information related to sponsoring/funding of the challenge. Also, state explicitly who had/will have access to the test case labels and when.

The challenge is not financially sponsored or supported by any company or entity. The data and the annotations are done within the DeepMIC project funded by the Bavarian Research Foundation with the cooperation partners OTH Regensburg, TU Munich and the company AKTORMed. The test data are only accessible to the challenge organizers and will not be made publicly available either during or after the end of the challenge.

## MISSION OF THE CHALLENGE

### Field(s) of application

State the main field(s) of application that the participating algorithms target.

Examples:

- Diagnosis
- Education
- Intervention assistance
- Intervention follow-up
- Intervention planning
- Prognosis
- Research
- Screening
- Training
- Cross-phase

Intervention assistance, Surgery, Research, Training

### Task category(ies)

State the task category(ies)

Examples:

- Classification
- Detection
- Localization
- Modeling
- Prediction

- Reconstruction
- Registration
- Retrieval
- Segmentation
- Tracking

## Segmentation, Localization, Classification, Tracking

### Cohorts

We distinguish between the target cohort and the challenge cohort. For example, a challenge could be designed around the task of medical instrument tracking in robotic kidney surgery. While the challenge could be based on ex vivo data obtained from a laparoscopic training environment with porcine organs (challenge cohort), the final biomedical application (i.e. robotic kidney surgery) would be targeted on real patients with certain characteristics defined by inclusion criteria such as restrictions regarding sex or age (target cohort).

a) Describe the target cohort, i.e. the subjects/objects from whom/which the data would be acquired in the final biomedical application.

**Patients undergoing laparoscopic cholecystectomy during real surgical interventions.**

b) Describe the challenge cohort, i.e. the subject(s)/object(s) from whom/which the challenge data was acquired.

Same as target cohort, with the restriction that the challenge data came from from the University Hospital rechts der Isar, Munich, Germany, the University Hospital Heidelberg, Heidelberg, Germany, and a smaller regional hospital near Munich, Munich, Germany.

### Imaging modality(ies)

Specify the imaging technique(s) applied in the challenge.

**Monocular endoscopic RGB video recordings**

### Context information

Provide additional information given along with the images. The information may correspond ...

a) ... directly to the image data (e.g. tumor volume).

**Frame-wise instance segmentation masks for surgical instrument parts together with the types of the instruments, keypoints for surgical instruments (tip point(s), shaft-tip transition point, shaft-point), surgical phase annotations on a per-frame basis.**

b) ... to the patient in general (e.g. sex, medical history).

**none**

### Target entity(ies)

a) Describe the data origin, i.e. the region(s)/part(s) of subject(s)/object(s) from whom/which the image data would be acquired in the final biomedical application (e.g. brain shown in computed tomography (CT) data, abdomen shown in laparoscopic video data, operating room shown in video data, thorax shown in fluoroscopy video). If necessary, differentiate between target and challenge cohort.

Abdomen shown in laparoscopic video data.

b) Describe the algorithm target, i.e. the structure(s)/subject(s)/object(s)/component(s) that the participating algorithms have been designed to focus on (e.g. tumor in the brain, tip of a medical instrument, nurse in an operating theater, catheter in a fluoroscopy scan). If necessary, differentiate between target and challenge cohort.

**Surgical instrument instance segmentations and keypoints. Phases of laparoscopic cholecystectomy.**

### Assessment aim(s)

Identify the property(ies) of the algorithms to be optimized to perform well in the challenge. If multiple properties are assessed, prioritize them (if appropriate). The properties should then be reflected in the metrics applied (see below, parameter metric(s)), and the priorities should be reflected in the ranking when combining multiple metrics that assess different properties.

- Example 1: Find highly accurate liver segmentation algorithm for CT images.
- Example 2: Find lung tumor detection algorithm with high sensitivity and specificity for mammography images.

Corresponding metrics are listed below (parameter metric(s)).

The challenge consists of three tasks: Instance segmentation and specification of the type of surgical instruments, determination of different keypoints, and prediction of the surgical phase. Depending on the task different aims of the submitted methods are expected: For instance segmentation, the most accurate pixel-wise labeling of the surgical instruments, including the correct classification of the tool types is the objective. For keypoint determination, the localization of the different keypoints (instrument tip(s), shaft-tip transition, shaft) represents the target. Regarding surgical phase recognition, the correct classification of the phase of the intervention for each individual frame is demanded. As the data involves real-world operations on humans, robust prediction of all these aspects is another key requirement for the algorithms.

## DATA SETS

### Data source(s)

a) Specify the device(s) used to acquire the challenge data. This includes details on the device(s) used to acquire the imaging data (e.g. manufacturer) as well as information on additional devices used for performance assessment (e.g. tracking system used in a surgical setting).

**Recordings from varying types of monocular endoscopic cameras.**

b) Describe relevant details on the imaging process/data acquisition for each acquisition device (e.g. image acquisition protocol(s)).

**The videos are from real-world human cholecystectomies from three surgical centers and were recorded during the operation**

c) Specify the center(s)/institute(s) in which the data was acquired and/or the data providing platform/source (e.g. previous challenge). If this information is not provided (e.g. for anonymization reasons), specify why.

The data originates from the University Hospital rechts der Isar, Munich, Germany (9 Videos), the University Hospital Heidelberg, Heidelberg, Germany (2 Videos), and a smaller regional hospital near Munich, Munich, Germany (2 Videos).

d) Describe relevant characteristics (e.g. level of expertise) of the subjects (e.g. surgeon)/objects (e.g. robot) involved in the data acquisition process (if any).

The cholecystectomies were performed by experienced surgeons with many years of professional experience.

### Training and test case characteristics

a) State what is meant by one case in this challenge. A case encompasses all data that is processed to produce one result that is compared to the corresponding reference result (i.e. the desired algorithm output).

Examples:

- Training and test cases both represent a CT image of a human brain. Training cases have a weak annotation (tumor present or not and tumor volume (if any)) while the test cases are annotated with the tumor contour (if any).
- A case refers to all information that is available for one particular patient in a specific study. This information always includes the image information as specified in data source(s) (see above) and may include context information (see above). Both training and test cases are annotated with survival (binary) 5 years after (first) image was taken.

A case corresponds to one frame of a video of a cholecystectomy. Regardless of whether the frame belongs to the training or test dataset, there are annotations for the instance segmentation of the surgical instruments and the type of tools, the coordinates of keypoints, and the surgical phase. The cases and annotations of the test data remain with the organizers and will not be released to the participants. One frame per second is annotated in each operation video and only these frames will be included in the evaluation. There are 13 videos in total, of which 9 come from one center and 2 each from the other two hospitals. To ensure a fair distribution, 6 videos from the first center and 1 video from each of the remaining centers are provided as training data.

b) State the total number of training, validation and test cases.

According to the division of the videos into 8 training and 5 test videos, the number of annotated frames corresponds to approx. 18,500 training images and 11,500 test images.

c) Explain why a total number of cases and the specific proportion of training, validation and test cases was chosen.

The split is the result of an equal division of the videos from the three clinics into training and test datasets. The number of annotated individual images is calculated based on the length of each video.

d) Mention further important characteristics of the training, validation and test cases (e.g. class distribution in classification tasks chosen according to real-world distribution vs. equal class distribution) and justify the choice.

The annotation of frames with the same time interval, i.e. one frame per second, is intended to cover all scenarios and ensure realistic conditions.

### Annotation characteristics

a) Describe the method for determining the reference annotation, i.e. the desired algorithm output. Provide the information separately for the training, validation and test cases if necessary. Possible methods include manual image annotation, in silico ground truth generation and annotation by automatic methods.

If human annotation was involved, state the number of annotators.

The annotations are made by a team of three people, consisting of two medical students and a professional surgeon with many years of experience who acts as annotator and supervisor.

b) Provide the instructions given to the annotators (if any) prior to the annotation. This may include description of a training phase with the software. Provide the information separately for the training, validation and test cases if necessary. Preferably, provide a link to the annotation protocol.

At the beginning of the annotations an annotation protocol was developed in close cooperation with the medical staff, which is currently being adapted to the status of the annotations, i.e. number of videos, frames, instrument classes, etc., and will be made available to the participants of the challenge when the website is published. The most important annotation rules are as follows: The "Computer Vision Annotation Tool (CVAT)" is used for annotation. For instance segmentation, the surgical instruments were outlined with polygons, assigning each surgical tool to one of a total of 20 predefined classes. Only what can be seen visually was annotated, i.e. no assumptions were made for hidden instruments behind organs and tissue or similar. If there are holes in the tools, for example, in the tip, these are seen as part of the instrument and not explicitly omitted. For superimposed instruments, there is a segmentation mask for each tool, i.e. a pixel can belong to several tools, as is usual for instance segmentation tasks. A video is always annotated by one annotator, and to ensure the high quality of the annotations, each annotated video is checked by another member of the team in a crossover procedure where polygons or instrument classes are adjusted if necessary. The annotations of the keypoints are created automatically based on the segmentations and subsequently checked for correctness by the human annotators. For the classification of the surgical phases, a video is divided into 7 parts based on timestamps, with frames between two timestamps belonging to one phase.

c) Provide details on the subject(s)/algorithm(s) that annotated the cases (e.g. information on level of expertise such as number of years of professional experience, medically-trained or not). Provide the information separately for the training, validation and test cases if necessary.

The annotations are made by a team of three people, consisting of two medical students and a professional surgeon with many years of experience who acts as annotator and supervisor.

d) Describe the method(s) used to merge multiple annotations for one case (if any). Provide the information separately for the training, validation and test cases if necessary.

No merging of annotations is applied.

### **Data pre-processing method(s)**

Describe the method(s) used for pre-processing the raw training data before it is provided to the participating teams. Provide the information separately for the training, validation and test cases if necessary.

The videos show human real-world cholecystectomies and are converted from .MOV to the .MP4 format. These videos will be made available to the participants of the challenge, together with a script to split the videos into individual frames, which can then be utilized by an algorithm. There will be no further pre-processing or manipulation of this raw data

### **Sources of error**

a) Describe the most relevant possible error sources related to the image annotation. If possible, estimate the magnitude (range) of these errors, using inter-and intra-annotator variability, for example. Provide the information separately for the training, validation and test cases, if necessary.

As the annotations were cross-corrected and supervised by a medical professional, no major sources of error are to be expected and inter-annotator variability should not have any effect. In scenarios with poor lighting scenarios, very fast movements of the instruments including recognizable movement artifacts or with a very heavily smeared camera lens, minimally inaccurate segmentation annotations may occur, but we estimate these to be insignificant.

b) In an analogous manner, describe and quantify other relevant sources of error.

NA

## ASSESSMENT METHODS

### Metric(s)

a) Define the metric(s) to assess a property of an algorithm. These metrics should reflect the desired algorithm properties described in assessment aim(s) (see above). State which metric(s) were used to compute the ranking(s) (if any).

- Example 1: Dice Similarity Coefficient (DSC)
- Example 2: Area under curve (AUC)

For the instance segmentation of the surgical instruments, three metrics are employed. For localization, the mean average precision (mAP) is applied, whereby the Mask Intersection over Union (IoU) is used as the localization criterion. The calculation of the mAP is analogous to that of the Common Objects in Context (COCO) dataset [1], i.e., the mAP is computed for IoU thresholds between 0.50 and 0.95 with an interval of 0.05 and the results are averaged for the final mAP [2]. As a per-class counting metric, the F1-score is applied, and the 95% Hausdorff-Distance (HD) serves as the boundary-based metric. For the assignment strategy of predictions to ground truth segmentations, the Hungarian Maximum Matching Algorithm is utilized.

The evaluation of the keypoint accuracy is analogous to the calculation of the COCO mAP, whereby the object keypoint similarity (OKS) is used instead of the mIoU [3]. The OKS is calculated using the Euclidean distance between a predicted and a ground truth point, which is passed through an unnormalized Gaussian distribution where the standard deviation corresponds to the square root of the size of the segmentation area multiplied by a per-keypoint constant. We use the tuned version of the OKS proposed by COCO, which is based on a per-keypoint standard deviation with respect to the object scale and an adjusted constant. A more detailed description of OKS and the tuned version is given in [3]. The classification of the surgical phases is evaluated using the Balanced Accuracy (BA) as the multi-class counting metric, the F1-score as the harmonic mean of precision of recall as the per-class counting metric, and the Area under the Receiver Operating Characteristic Curve (AUROC) as the threshold-based metric.

1: Lin, Tsung-Yi, Michael Maire, Serge J. Belongie, James Hays, Pietro Perona, Deva Ramanan, Piotr Dollár and C. Lawrence Zitnick. "Microsoft COCO: Common Objects in Context." European Conference on Computer Vision (2014).

2: Common Objects in Context - Detection Evaluation. <https://cocodataset.org/detection-eval>. Accessed: 14 November 2023.

3: Common Objects in Context - Keypoint Evaluation. <https://cocodataset.org/keypoints-eval>. Accessed: 14 November 2023.

b) Justify why the metric(s) was/were chosen, preferably with reference to the biomedical application.

The metrics mAP, F1-score, and 95% HD for instance segmentation of surgical tools were selected based on the publication by Maier-Hein et al. [1]. Furthermore, these metrics are common and frequently used for instance segmentation and are widely accepted in the community as measures for the quality of an algorithm. The COCO variant of mAP also serves to ensure that algorithms whose predictions have a higher IoU benefit more from it and that a higher IoU has a greater impact on the final result. Analogously, the calculation of the mAP based on the OKS for the keypoint estimation task as a measure of the quality of an algorithm should lead to the most accurate possible determination of keypoint coordinates, with similar benefits as mentioned above. The metrics BA, F1-score, and AUROC for the classification of procedure phases were also selected based on [1], which represent widely used metrics for classification tasks and ensure a reliable statement about the quality of a method.

[1] Maier-Hein, L. et al. "Metrics reloaded: Pitfalls and recommendations for image analysis validation." arXiv. org 2206.01653 (2022).

### Ranking method(s)

a) Describe the method used to compute a performance rank for all submitted algorithms based on the generated metric results on the test cases. Typically the text will describe how results obtained per case and metric are aggregated to arrive at a final score/ranking.

By determining the results per video and averaging them we give equal weighting to all videos, even if they are of different lengths. The same applies to the task of phase classification in videos regarding the varying number of frames in a phase.

b) Describe the method(s) used to manage submissions with missing results on test cases.

As participants submit docker containers containing their algorithms, there should be a corresponding result for each test case. However, if a result is missing, the metrics for this case will be set to zero.

c) Justify why the described ranking scheme(s) was/were used.

We calculate the above mentioned metrics for each class in a frame, and average the results across all classes to get a final result for the single frame. We carry out this procedure for all images in a video to get a per-video result and average the results over all videos in the test dataset. For the phase classification task, we additionally average the per-phase results over all phases in a video to ensure that an unbalanced number of frames between phases does not affect the overall result. Since our challenge consists of three different tasks, and participants do not necessarily have to take part in all tasks, we carry out a separate evaluation and obtain three result lists at the end. For each task, we calculate all mentioned metrics and average the corresponding ranks in order to determine the final task-specific rank.

### Statistical analyses

a) Provide details for the statistical methods used in the scope of the challenge analysis. This may include

- description of the missing data handling,
- details about the assessment of variability of rankings,
- description of any method used to assess whether the data met the assumptions, required for the particular statistical approach, or
- indication of any software product that was used for all data analysis methods.

We apply statistical methods such as bootstrapping and the Wilcoxon signed rank test to determine the stability of the rankings and the significance of the differences between the submitted algorithms. The statistical analysis will be done with a self-coded python script, cross-checked by an experienced mathematician.

b) Justify why the described statistical method(s) was/were used.

In [1], Maier-Hein et al. identify these methods as suitable for determining rank variability.

[1] Maier-Hein, L., Eisenmann, M., Reinke, A. et al. Why rankings of biomedical image analysis competitions should be interpreted with care. Nat Commun 9, 5217 (2018). <https://doi.org/10.1038/s41467-018-07619-7>

### Further analyses

Present further analyses to be performed (if applicable), e.g. related to

- combining algorithms via ensembling,
- inter-algorithm variability,
- common problems/biases of the submitted methods, or
- ranking variability.

In addition to the metrics mentioned above, the inference runtime of each algorithm is specified in the final paper, which has no influence on the ranking procedure.
